# Supplementary material for: Datasets, Models, and Algorithms for Multi-Sensor, Multi-agent Autonomy Using AVstack
Source: arXiv:2312.04970 source file (2023-12-08)
Supplement: Supplementary file 1 [file 99-appendix-1.tex]

%%%%%%%%%%%%%%%%%%%%%%%%%%%%%%%%%%%%%%%%%%%%%%%%%%%%%%%%%%%%%%%%%%%%%%%%%%%%%%%%
\section*{APPENDIX}

Appendixes should appear before the acknowledgment.
